# Supplementary material for: User-in-the-loop Evaluation of Multimodal LLMs for Activity Assistance
Source: arXiv:2408.03160 source file (2024-08-12)
Supplement: Supplementary file 1 [file EK55_7B.tex]

\begin{table}[t]
\centering
\scriptsize
\begin{tabular}{lcccc}
\multicolumn{1}{l|}{Method} & \multicolumn{1}{c|}{Modality} & Prompt & Visual feature      & Accuracy   \\ \hline
\multicolumn{1}{l|}{Socratic} & \multicolumn{1}{c|}{T}   & Caption  &    & 8.4       \\
\multicolumn{1}{l|}{VCLM 13B} & \multicolumn{1}{c|}{V+T}  &  Caption  & Internvideo   & 11.88       \\
\multicolumn{1}{l|}{VCLM aligned} & \multicolumn{1}{c|}{V+T}  &  Caption  & Internvideo   & 3.9       \\
\multicolumn{1}{l|}{VCLM interleaved} & \multicolumn{1}{c|}{V+T}  &  Caption  & TimeSformer  & 1.2       \\
\hline
\multicolumn{1}{l|}{Socratic} & \multicolumn{1}{c|}{T}   &  GT action &    & 13.7       \\
\multicolumn{1}{l|}{VCLM 13B} & \multicolumn{1}{c|}{V+T}  &   GT action & Internvideo   & 12.87       \\
\multicolumn{1}{l|}{VCLM aligned} & \multicolumn{1}{c|}{V+T}  &   GT action & Internvideo   & 11.9       \\
\multicolumn{1}{l|}{VCLM interleaved} & \multicolumn{1}{c|}{V+T}  &  GT action  & TimeSformer  & 4.3       \\
\hline
\end{tabular}
\caption{\textbf{Next action prediction on the EK-55. }
}
\label{tab:aria}
\end{table}
