# Supplementary material for: User-in-the-loop Evaluation of Multimodal LLMs for Activity Assistance
Source: arXiv:2408.03160 source file (2024-08-12)
Supplement: Supplementary file 2 [file aria_7B.tex]

\begin{table}[t]
\centering
\scriptsize
\begin{tabular}{lccc}
\multicolumn{1}{l|}{Method} & \multicolumn{1}{c|}{Modality}  & Visual feature      & BERT score   \\ \hline
\multicolumn{1}{l|}{Socratic} & \multicolumn{1}{c|}{T}      &    & 0.615       \\
\multicolumn{1}{l|}{VCLM aligned} & \multicolumn{1}{c|}{V+T}      & Internvideo  & 0.613       \\
\multicolumn{1}{l|}{VCLM interleaved} & \multicolumn{1}{c|}{V+T}      & TimeSformer  & 0.611       \\
\hline
\end{tabular}
\caption{\textbf{Next action caption prediction on the Aria data.}
}
\label{tab:aria}
\end{table}
