# Supplementary material for: User-in-the-loop Evaluation of Multimodal LLMs for Activity Assistance
Source: arXiv:2408.03160 source file (2024-08-12)
Supplement: Supplementary file 3 [file lta_7B.tex]

\begin{table}[t]
\centering
\scriptsize
\begin{tabular}{l|cclll}
\multicolumn{1}{c}{} &  &  & \multicolumn{3}{c}{ED@(Z=20)}  \\ \hline
\multicolumn{1}{l}{Method}   &  Modality & Visual feature & Verb   & Noun    & Action \\ \hline
\multicolumn{1}{l}{SlowFast\cite{grauman2022ego4d}} & V &   & 0.745  & 0.779   & 0.941       \\ 
\multicolumn{1}{l}{Socratic} & T  && 0.731  & 0.812   & 0.951       \\ 
\multicolumn{1}{l}{AntGPT\cite{zhao2023antgpt}} & T  && 0.702  & 0.702   & 0.912       \\ 
\multicolumn{1}{l}{Palm \cite{huang2023palm}} & T  &  & 0.695  & 0.650   & 0.885    \\ 
\hline
\multicolumn{1}{l}{VCLM aligned} & V+T  & Internvideo & 0.792  & 0.765   & 0.958      \\ 
\multicolumn{1}{l}{VCLM interleaved} & V+T  &TimeSformer  & 0.823  & 0.775   & 0.963      \\ 
\multicolumn{1}{l}{VLaMP \cite{patel2023pretrained}} & V+T  & S3D & 0.730  & 0.772   & 0.932    \\ 
\multicolumn{1}{l}{VideoLLM \cite{chen2023videollm}} & V+T  &  & 0.717  & 0.736   & 0.925    \\ 
%\multicolumn{1}{l}{ICVAE \cite{mascaro2022intention}} & V+T  &  & 0.741  & 0.739   & 0.930   not LLM   \\ 
\hline
\end{tabular}
\caption{\textbf{Results of the Ego4D long-term action anticipation task Val set. Lower is better. Add GT history numbers?}
}
\label{tab:long_term_results}
\end{table}
