# Supplementary material for: User-in-the-loop Evaluation of Multimodal LLMs for Activity Assistance
Source: arXiv:2408.03160 source file (2024-08-12)
Supplement: Supplementary file 4 [file vpa_7B.tex]

% Please add the following required packages to your document preamble:
% \usepackage{booktabs}
% \usepackage{multirow}
% \usepackage{graphicx}
% \begin{table}[]
% \centering
% \setlength{\tabcolsep}{3pt}
% \resizebox{\columnwidth}{!}{%
% \begin{tabular}{@{}llrrrrrrr@{}}
% \toprule
% \multirow{2}{*}{\textbf{Data}} &
%   \multirow{2}{*}{\textbf{Model}} &
%   $l=1$ &
%   \multicolumn{3}{c}{$l=3$} &
%   \multicolumn{3}{c}{$l=4$} \\ \cmidrule(l){3-9} 
%  &
%    &
%   \{n/m\}Acc &
%   SR &
%   mAcc &
%   mIOU &
%   SR &
%   mAcc &
%   mIOU \\ \midrule
% \multirow{4}{*}{\begin{tabular}[c]{@{}l@{}}Cross-\\ task\end{tabular}} &
%   {Random} &
%   0.9   &
%   0.0   &
%   0.9   &
%   1.5   &
%   0.0   &
%   0.9   &
%   1.9  \\
%  &
%   VCLM &
%   29.0   &
%   7.0    &
%   25.8   &
%   41.1   &
%    2.8   &
%     22.9 &
%   42.9  \\
%  &
%   Socratic &
%    27.2   &
%   5.7     &
%    24.3   &
%    40.8   &
%   3.5    &
%   23.8   &
%   44.0   \\
%   \hline
%  &
%   \color{gray}{VLaMP (supervised)} &
%   \color{gray}{50.6} &
%   \color{gray}{10.3} &
%   \color{gray}{35.3} &
%   \color{gray}{44.0} &
%   \color{gray}{4.4} &
%   \color{gray}{31.7} &
%   \color{gray}{43.4} \\ 
%   \bottomrule
% \end{tabular}%
% }
% \caption{\textbf{Performance on CrossTask VPA. } }
% \label{tab:main-results-vlamp}
% \end{table}

% Please add the following required packages to your document preamble:
% \usepackage{booktabs}
% \usepackage{multirow}
% \usepackage{graphicx}
\begin{table}[]
\centering
\setlength{\tabcolsep}{3pt}
\resizebox{\columnwidth}{!}{%
\begin{tabular}{@{}llrrrrrrr@{}}
\toprule
\multirow{2}{*}{\textbf{Data}} &
  \multirow{2}{*}{\textbf{Model}} &
  $l=1$ &
  \multicolumn{3}{c}{$l=3$} &
  \multicolumn{3}{c}{$l=4$} \\ \cmidrule(l){3-9} 
 &
   &
  \{n/m\}Acc &
  SR &
  mAcc &
  mIOU &
  SR &
  mAcc &
  mIOU \\ \midrule
\multirow{4}{*}{\begin{tabular}[c]{@{}l@{}}Cross-\\ task\end{tabular}} &
  {Random} &
  0.9   &
  0.0   &
  0.9   &
  1.5   &
  0.0   &
  0.9   &
  1.9  \\
 &
  Socratic &
  29.0   &
  7.0    &
  25.8   &
  41.1   &
   2.8   &
    22.9 &
  42.9  \\
 &
  VCLM alinged 7B &
   27.2   &
  5.7     &
   24.3   &
   40.8   &
  3.5    &
  23.8   &
  44.0   \\
 &
  VCLM interleaved &
  26.4  &
   5.5   &
  21.3 &
  36.2  &
    3.3  &
    21.7 &
  40.4  \\
  \hline
 &
  \color{gray}{VLaMP (supervised)} &
  \color{gray}{50.6} &
  \color{gray}{10.3} &
  \color{gray}{35.3} &
  \color{gray}{44.0} &
  \color{gray}{4.4} &
  \color{gray}{31.7} &
  \color{gray}{43.4} \\ 
  \bottomrule
\end{tabular}%
}
\caption{\textbf{Performance on CrossTask VPA. add number of shots, finetuned (which part?, LLM) or not, supervision} }
\label{tab:main-results-vlamp}
\end{table}
